# Supplementary material for: Combined investigation of collective amplitude and phase modes in a quasi-one-dimensional charge-density-wave system over a wide spectral range
Source: arXiv:2303.08558 source file (2023-03-15)
Supplement: Supplementary file 2 [file header_suppl.tex]

%\usepackage[pdftex]{graphics}
\usepackage{graphicx}
%\usepackage{float}
\usepackage{amsmath}
\usepackage{amssymb}
%\usepackage{comment}
\usepackage{xspace}
\usepackage{xcolor} 
%\usepackage{cleveref}
\usepackage{upgreek}
\usepackage{multirow}

%\usepackage{jabbrv}

\usepackage[utf8]{inputenc}

\newcommand{\beq}{\begin{equation}}
\newcommand{\eeq}{\end{equation}}

% General Helpers
\usepackage{pgffor} % To support \foreach coommand in macros
\DeclareRobustCommand{\chem}[1]{%
\ensuremath{\foreach \x/\y in {#1} {{\mathrm{\x}_{\y}}}}\xspace}

\newcommand{\usr}[2]{\ensuremath{#1_{\mathrm{#2}}}\xspace} % 

% Materials
\newcommand{\kmo}{\chem{K/0.3,Mo/,O/3}}

% Units
\newcommand{\unit}[1]{\ensuremath{\,{\mathrm{#1}}}\xspace}
\newcommand{\pcm}{\ensuremath{\,\mathrm{cm}^{-1}}\xspace}
%\newcommand{\mum}{\ensuremath{\,\upmu\textrm{m}}\xspace}
%\newcommand{\muJ}{\unit{\upmu J}}
\newcommand{\mum}{\unit{\mu m}}
\newcommand{\muJ}{\unit{\mu J}}
\newcommand{\fsec}{\unit{fs}}
\newcommand{\psec}{\unit{ps}}
\newcommand{\Hz}{\unit{Hz}}
\newcommand{\kHz}{\unit{kHz}}
\newcommand{\GHz}{\unit{GHz}}
\newcommand{\THz}{\unit{THz}}
\newcommand{\Kel}{\ensuremath{\,\mathrm{K}}}
\newcommand{\nm}{\unit{nm}}
\newcommand{\mm}{\unit{mm}}

\newcommand{\tisa}{Ti:Al$_2$O$_3$\xspace}

% Misc
\newcommand{\rarr}{\ensuremath{\rightarrow}\xspace}
\newcommand{\simx}{{\sim}}

% Quantities
\newcommand{\kF}{\usr{k}{F}\xspace}
\newcommand{\epsr}[1]{\usr{\varepsilon}{#1}\xspace}
\newcommand{\nuzn}{\ensuremath{\nu_{0n}}\xspace}
\newcommand{\nuznA}{\ensuremath{\nu_{0n}^{(A)}}\xspace}
\newcommand{\nuznP}{\ensuremath{\nu_{0n}^{(P)}}\xspace}
\newcommand{\nuzA}{\ensuremath{\nu_{01}^{(A)}}\xspace}
\newcommand{\nuzP}{\ensuremath{\nu_{01}^{(P)}}\xspace}

%\newcommand{\wznA}{\ensuremath{\omega_{0n}^{(A)}}\xspace}
%\newcommand{\wznP}{\ensuremath{\omega_{0n}^{(P)}}\xspace}
%\newcommand{\wzA}{\ensuremath{\omega_{01}^{(A)}}\xspace}
\newcommand{\wzP}{\ensuremath{\omega_{01}^{(P)}}\xspace}


\newcommand{\wzn}{\ensuremath{\omega_{0n}}\xspace}
\newcommand{\Wzn}{\ensuremath{\Omega_{0n}}\xspace} % Bare mode frequencies
%\newcommand{\Wz}[1]{\ensuremath{\Omega_{0#1}}\xspace} % Bare mode frequencies
\newcommand{\Gamn}{\ensuremath{\Gamma_{n}}\xspace}
\newcommand{\phin}{\ensuremath{\varphi_{0n}}\xspace}
\newcommand{\Wpin}{\usr{\Omega}{p}}
\newcommand{\Upin}{\usr{U}{p}}
\newcommand{\Upinx}{\usr{U}{p}^{(1)}}


% Commments
% \newcommand{\HGR}[1]{\textcolor{orange}{[#1]}}
% \newcommand{\HR}[1]{\textcolor{red}{#1}}
\newcommand{\KW}[1]{\textcolor{blue}{[KW: #1]}}
\newcommand{\KWx}[1]{\textcolor{blue}{#1}}
\newcommand{\MDT}[1]{\textcolor{purple}{[MDT: #1]}}
%\newcommand{\toKW}[1]{\textcolor{\red}{[$\rightarrow$ KW: #1]}}

% Affiliations
\newcommand{\ffm}{Physikalisches Institut, J. W. Goethe-Universität, D-60438 Frankfurt am Main, Germany} 
\newcommand{\jgu}{Institute of Physics, Johannes Gutenberg-University Mainz, D-55128 Mainz, Germany}

% For Supplmentary
% Ensure everthing above can be updated by over-pasting from main paper
%\newcommand{\chi_n}{\ensuremath{\nu_{01}^{(A)}}\xspace}
\newcommand{\Tc}{\usr{T}{c}}
\newcommand{\Tcz}{\usr{T}{c0}}
